# Supplementary material for: Algorithmic Persuasion Through Simulation
Source: arXiv:2311.18138 source file (2025-02-12)
Supplement: Supplementary file 1 [file prompts.tex]

\section{Example GPT-4 prompts and responses}\label{app:gpt4}
This section contains three examples of GPT-4 performing correct Bayesian reasoning for a simple persuasion task. 
All three replies were generated in the same session and little to no prompt engineering was required. 
While GPT-4's replies have been edited for formatting, their contents have not been changed. 
\subsection{Example 1: seedy-looking alley}
\textbf{Prompt:} 
You are in a seedy-looking alley and somebody comes up to you and offers to sell you a designer bag. The bag is either fake or real. You believe that there is some probability that the bag is fake, and some probability that the bag is real. Use your knowledge about how often real designer bags are bought and sold in seedy-looking alleys to infer this probability.

If you purchase the bag and it is real, you receive a reward of 1. If you purchase the bag and it is fake, you receive a reward of -1. Otherwise, you receive a reward of 0. Your only goal is to maximize your expected reward.

I know whether the used bag is real or fake. I will give you a recommendation, and then you will then decide whether or not to purchase the bag. If the bag is real, I will always recommend that you purchase the bag. If the bag is fake, with 25\% probability I will recommend that you purchase the bag. The other 75\% of the time I will recommend that you do not purchase the bag.

I recommend that you purchase the bag. What is your decision?

\textbf{GPT-4 reply:}
To solve this problem, we can use Bayes' Theorem to update our beliefs based on the new evidence provided by the recommendation to purchase the bag. Let's denote:

\begin{itemize}
    \item \(P(\text{Real})\) as the prior probability that the bag is real.
    \item \(P(\text{Fake})\) as the prior probability that the bag is fake. Given the context, we assume \(P(\text{Fake}) = 1 - P(\text{Real})\).
    \item \(P(\text{Recommend}|\text{Real})\) as the probability of getting a recommendation to purchase the bag given that it is real, which is 1 (since the condition states that if the bag is real, I will always recommend that you purchase it).
    \item \(P(\text{Recommend}|\text{Fake})\) as the probability of getting a recommendation to purchase the bag given that it is fake, which is 0.25.
\end{itemize}

The problem asks us to decide whether to purchase the bag based on the recommendation to do so, aiming to maximize the expected reward. To make this decision, we need to calculate the posterior probability that the bag is real given the recommendation, \(P(\text{Real}|\text{Recommend})\), and compare the expected rewards.

The expected reward for purchasing the bag is:

\[E(\text{Purchase}) = P(\text{Real}|\text{Recommend}) \times 1 + P(\text{Fake}|\text{Recommend}) \times (-1)\]

Where:
\[P(\text{Real}|\text{Recommend}) = \frac{P(\text{Recommend}|\text{Real}) \times P(\text{Real})}{P(\text{Recommend})}\]

And:
\[P(\text{Recommend}) = P(\text{Recommend}|\text{Real}) \times P(\text{Real}) + P(\text{Recommend}|\text{Fake}) \times P(\text{Fake})\]

Given the setting does not specify the prior probability \(P(\text{Real})\), we need to make an assumption. It's reasonable to assume that the prior probability \(P(\text{Real})\) is low in a seedy-looking alley, but for calculation purposes, let's assign a hypothetical value to \(P(\text{Real})\). 

Let's assume \(P(\text{Real}) = 0.1\) (or 10\%) as a starting point, indicating that there's a low but not impossible chance the bag sold in such a context is real. This is purely illustrative; the actual prior would depend on more specific information about the prevalence of real vs. fake designer bags in such contexts.

Let's calculate the posterior probability \(P(\text{Real}|\text{Recommend})\) with this assumption and determine the expected reward to decide whether to purchase the bag.

Based on the calculation, the posterior probability that the bag is real given the recommendation to purchase it is approximately 30.77\%. The expected reward for purchasing the bag, considering this probability, turns out to be approximately -0.38. 

Given that the goal is to maximize the expected reward, and purchasing the bag results in a negative expected reward, the optimal decision under these assumptions would be \textbf{not to purchase the bag}. This decision is based on the calculated expected reward, which suggests that the risk of the bag being fake (and thus incurring a negative reward) outweighs the potential benefit of it being real.
\subsection{Example 2: fancy designer store}
\textbf{Prompt:} 
You are in a fancy designer store and somebody comes up to you and offers to sell you a designer bag. The bag is either fake or real. You believe that there is some probability that the bag is fake, and some probability that the bag is real. Use your knowledge about how often real designer bags are bought and sold in fancy designer stores to infer this probability.

If you purchase the bag and it is real, you receive a reward of 1. If you purchase the bag and it is fake, you receive a reward of -1. Otherwise, you receive a reward of 0. Your only goal is to maximize your expected reward.

I know whether the used bag is real or fake. I will give you a recommendation, and then you will then decide whether or not to purchase the bag. If the bag is real, I will always recommend that you purchase the bag. If the bag is fake, with 25\% probability I will recommend that you purchase the bag. The other 75\% of the time I will recommend that you do not purchase the bag.

I recommend that you purchase the bag. What is your decision?

\textbf{GPT-4 reply:}
To update our decision based on the new context of being in a fancy designer store, we need to adjust our prior probability to reflect the likelihood that a bag sold in such a setting is real. The probability of encountering a real designer bag in a fancy designer store is significantly higher than in a seedy-looking alley. Thus, \(P(\text{Real})\) should be adjusted upwards.

Let's assume \(P(\text{Real}) = 0.9\) for this scenario, reflecting a high likelihood that bags sold in fancy designer stores are authentic. This is a reasonable assumption given the context, but the actual value could vary based on more specific information about the store and its reputation for authenticity.

With the updated prior probability, let's recalculate the posterior probability \(P(\text{Real}|\text{Recommend})\) given the recommendation to purchase the bag and determine the expected reward to decide whether to purchase the bag under these new conditions.

In the context of being in a fancy designer store, the posterior probability that the bag is real, given the recommendation to purchase it, is approximately 97.30\%. The expected reward for purchasing the bag, considering this probability, is approximately 0.95.

Given that the goal is to maximize the expected reward, and purchasing the bag results in a positive expected reward, the optimal decision under these assumptions would be \textbf{to purchase the bag}. This decision is based on the calculated expected reward, which suggests that the likelihood of the bag being real (and thus incurring a positive reward) significantly outweighs the risk of it being fake.

\subsection{Example 3: crowded street market}
\textbf{Prompt:} 
You are in the middle of a crowded street market and somebody comes up to you and offers to sell you a designer bag. The bag is either fake or real. You believe that there is some probability that the bag is fake, and some probability that the bag is real. Use your knowledge about how often real designer bags are bought and sold in street markets to infer this probability.

If you purchase the bag and it is real, you receive a reward of 1. If you purchase the bag and it is fake, you receive a reward of -1. Otherwise, you receive a reward of 0. Your only goal is to maximize your expected reward.

I know whether the used bag is real or fake. I will give you a recommendation, and then you will then decide whether or not to purchase the bag. If the bag is real, I will always recommend that you purchase the bag. If the bag is fake, with 25\% probability I will recommend that you purchase the bag. The other 75\% of the time I will recommend that you do not purchase the bag.

I recommend that you purchase the bag. What is your decision?

\textbf{GPT-4 reply:}
In the context of a crowded street market, the prior probability that a designer bag offered for sale is real (i.e., \(P(\text{Real})\)) may be lower than in a fancy designer store but potentially higher than in a seedy-looking alley. The likelihood of encountering genuine designer goods in street markets can vary widely based on the specific market and its reputation, but generally, there's a significant risk of counterfeits. Let's assume \(P(\text{Real}) = 0.5\) as a neutral starting point, acknowledging this context's ambiguity.

Given:
\begin{itemize}
    \item \(P(\text{Real}) = 0.5\), reflecting an uncertain mix of real and fake goods commonly found in street markets.
    \item \(P(\text{Fake}) = 1 - P(\text{Real})\), naturally.
    \item \(P(\text{Recommend}|\text{Real}) = 1\), as if the bag is real, the recommendation to purchase is certain.
    \item \(P(\text{Recommend}|\text{Fake}) = 0.25\), reflecting the given probability of recommending the purchase even if the bag is fake.
\end{itemize}

We'll calculate the posterior probability \(P(\text{Real}|\text{Recommend})\) with these values to determine whether the recommendation to purchase the bag increases the likelihood of it being real enough to justify a purchase. Let's also determine the expected reward based on this probability.

In the context of a crowded street market, the posterior probability that the bag is real, given the recommendation to purchase it, is approximately 80\%. The expected reward for purchasing the bag, considering this probability, is about 0.6.

Given the goal is to maximize the expected reward, and purchasing the bag results in a positive expected reward, the optimal decision under these assumptions would be \textbf{to purchase the bag}. This decision is based on the calculated expected reward, which suggests that the likelihood of the bag being real (and thus incurring a positive reward) outweighs the risk of it being fake in the context of a street market, especially following a recommendation to purchase.
