# Supplementary material for: Algorithmic Persuasion Through Simulation
Source: arXiv:2311.18138 source file (2025-02-12)
Supplement: Supplementary file 2 [file regret.tex]

\subsection{Regret Analysis}
\begin{definition}[Regret]
    Let $N$ be the number of time-steps, $\cP_{\tau^*}$ be the distribution over types which is a point mass at the true type $\tau^*$, $\sigma^*$ be the corresponding optimal messaging policy, and $\sigma_n$ be the messaging policy played by the sender at time $n$. 
    The sender's regret is given by 
    \begin{equation*}
        R(N) := \sum_{n=1}^N V(\cP_{\tau^*}, \sigma^*) - V(\cP_{\tau^*}, \sigma_n).
    \end{equation*}
\end{definition}
\begin{corollary}
    The following procedure obtains expected regret $\mathbb{E}[R(N)] = O(\log N)$: Run~\Cref{alg:total} with $\epsilon = \gamma = 1/N$ and $K = \log N$, then message according to the resulting messaging policy $\sigma_K$ for the remaining $N - \log N$ time-steps.
\end{corollary}
\begin{proof}
    Consider running~\Cref{alg:total} for $K = O(\log(1/\epsilon))$ queries, where $\epsilon$ is left unspecified for now. 
    \begin{equation*}
    \begin{aligned}
        R(N) &:= \sum_{n=1}^N V(\cP_{\tau^*}, \sigma^*) - V(\cP_{\tau^*}, \sigma_n)\\
        &\leq O(N\epsilon \log(1/\gamma)) + \sum_{n=1}^N V(\cP'_{\tau^*}, \sigma') - V(\cP'_{\tau^*}, \sigma_n)\\
        &\leq O(N\epsilon \log(1/\gamma)) + O(\log(1/\epsilon)) + \sum_{n=1}^N V(\cP'_{\tau^*}, \sigma') - V(\cP'_{\tau^*}, \Tilde{\sigma})\\
        &= O(N\epsilon \log(1/\gamma)) + O(\log(1/\epsilon)) + N(V(\cP'_{\tau^*}, \sigma') - V(\Tilde{\cP}_{\tau^*}, \Tilde{\sigma}) + V(\Tilde{\cP}_{\tau^*}, \Tilde{\sigma}) - V(\cP'_{\tau^*}, \Tilde{\sigma})).
    \end{aligned}
    \end{equation*}
    with probability at least $1 - \gamma$, 
    where $\cP'_{\tau^*}$ is the probability distribution which is a point mass on the optimal type in $\cT'$ and $\Tilde{\cP}_{\tau^*}$ is the probability distribution which is a point mass on the optimal type in $\Tilde{\cT}$ and $\sigma'$ and $\Tilde{\sigma}$ are the respective optimal messaging policies for those types. 
    The first inequality follows from a line of reasoning similar to the proof of~\Cref{thm:approx.algorithm} and the second follows from the fact that utilities are bounded by $1$. 
    By~\Cref{prop:value.monotone.prob}, we know that $V(\cP'_{\tau^*}, \sigma') - V(\Tilde{\cP}_{\tau^*}, \Tilde{\sigma}) = O(\epsilon)$, since $\cP'_{\tau^*}$ is a ``rounded up'' version of $\Tilde{\cP}_{\tau^*}$. 
    Similarly, we also know that $V(\Tilde{\cP}_{\tau^*}, \Tilde{\sigma}) - V(\cP'_{\tau^*}, \Tilde{\sigma}) \leq 0$ by~\Cref{prop:value.monotone.prob}. 
    Finally, we obtain the desired result by setting $\epsilon = \gamma = 1/N$. 
\end{proof}
