# Supplementary material for: Algorithmic Persuasion Through Simulation
Source: arXiv:2311.18138 source file (2025-02-12)
Supplement: Supplementary file 4 [file further_background.tex]

\onecolumn
\section{Further Background}
% \xhdr{Remarks.}
%
