# Supplementary material for: Algorithmic Persuasion Through Simulation
Source: arXiv:2311.18138 source file (2025-02-12)
Supplement: Supplementary file 5 [file setting-app.tex]

\section{Appendix for~\Cref{sec:setting}: Model}\label{app:model}
\rp*
